# Supplementary material for: Auto-Encoding Variational Bayes for Inferring Topics and Visualization
Source: arXiv:2010.09233 source file (2020-10-25)
Supplement: Supplementary file 1 [file appendix.tex]

% \section{Appendix}
% \subsection{Approximation of the Reconstruction Term}

% $$
% \begin{aligned}
% &\mathbb{E}_{q\left(\mathbf{Z} | \mathcal{D}\right)}\left[\log p\left(\mathcal{D} | \mathbf{Z}\right)\right] 
% \\&=\int q\left(\mathbf{Z} | \mathcal{D}\right)\left[\log p\left(\mathcal{D} | \mathbf{Z}\right)\right] \mathrm{d} Z \\
% &=\int \frac{1}{N} \sum_{i=1}^{N} q\left(\mathbf{x} | \boldsymbol{w}^{(i)}\right) q\left(\mathbf{\beta} | \boldsymbol{D}\right) q\left(\mathbf{\phi} | \boldsymbol{D}\right) \left[\log p\left(\mathcal{D} | \mathbf{Z}\right)\right] \mathrm{d} \boldsymbol{Z} \\
% &=\frac{1}{N} \sum_{i=1}^{N} \int q\left(\mathbf{x} | \boldsymbol{w}^{(i)}\right) q\left(\mathbf{\beta} | \boldsymbol{D}\right) q\left(\mathbf{\phi} | \boldsymbol{D}\right) \left[\log p\left(\mathcal{D} | \mathbf{Z}\right)\right] \mathrm{d} \boldsymbol{Z} \\
% &=\frac{1}{N} \sum_{i=1}^{N} \mathbb{E}_{ q\left(\mathbf{x} | \boldsymbol{w}^{(i)}\right) q\left(\mathbf{\beta} | \boldsymbol{D}\right) q\left(\mathbf{\phi} | \boldsymbol{D}\right) }\left[\log p\left(\mathcal{D} | \mathbf{Z}\right)\right]
% \end{aligned}
% $$


% $$
% \log p\left(\mathcal{D} | \mathbf{Z}\right)=\log \prod_{j=1}^{N} p\left(\boldsymbol{w}^{(j)} | \mathbf{Z}\right)=\sum_{j=1}^{N} \log p\left(\boldsymbol{w}^{(j)} | \mathbf{Z}\right)
% $$
% Substituting this into the reconstruction term, we have:


% $$
% \begin{aligned}
% &\mathbb{E}_{q\left(\mathbf{Z} | \mathcal{D}\right)}\left[\log p\left(\mathcal{D} | \mathbf{Z}\right)\right]
% \\
% &=\frac{1}{N} \sum_{i=1}^{N} \mathbb{E}_{q\left(\mathbf{x} | \boldsymbol{w}^{(i)}\right) q\left(\mathbf{\beta} | \boldsymbol{D}\right) q\left(\mathbf{\phi} | \boldsymbol{D}\right)}\left[\sum_{j=1}^{N} \log p\left(\boldsymbol{w}^{(j)} | \mathbf{Z}\right)\right]
% \end{aligned}
% $$

% $$
% \begin{aligned}
% &\mathbb{E}_{q\left(\mathbf{Z} | \mathcal{D}\right)}\left[\log p\left(\mathcal{D} | \mathbf{Z}\right)\right]
% \\&=\sum_{i=1}^{N} \mathbb{E}_{q\left(\mathbf{x} | \boldsymbol{w}^{(i)}\right) q\left(\mathbf{\beta} | \boldsymbol{D}\right) q\left(\mathbf{\phi} | \boldsymbol{D}\right)}\left[\frac{1}{N} \sum_{j=1}^{N} \log p\left(\boldsymbol{w}^{(j)} | \mathbf{Z}\right)\right]
% \end{aligned}
% $$

% and apply Jensen inequality for the special case of log, i.e.
% $$
% \log \left(\frac{1}{N} \sum_{i=1}^{N} a_{i}\right) \geq \frac{1}{N} \sum_{i=1}^{N} \log \left(a_{i}\right)
% $$

% $$
% \begin{aligned}
% &\mathbb{E}_{q\left(\mathbf{Z} | \mathcal{D}\right)}\left[\log p\left(\mathcal{D} | \mathbf{Z}\right)\right] 
% \\&\leq \sum_{i=1}^{N} \mathbb{E}_{q\left(\mathbf{x} | \boldsymbol{w}^{(i)}\right) q\left(\mathbf{\beta} | \boldsymbol{D}\right) q\left(\mathbf{\phi} | \boldsymbol{D}\right)}\left[\log \left(\frac{1}{N} \sum_{j=1}^{N} p\left(\boldsymbol{w}^{(j)} | \mathbf{Z}\right)\right)\right]
% \end{aligned}
% $$

% Assume that the likelihood $p\left(\boldsymbol{w}^{(j)} | \mathbf{Z}\right)$ representing the probability of a reconstructed sample from a latent code $Z$ imitating the sample $w^{(j)}$ will only be non-zero if $Z$ is sampled from the embedding prediction distribution with the same sample $w^{(j)}$ at the encoder input. With this assumption, $N-1$ posterior distributions in the inner summation will be dropped as zeros and the only non-zero term is $p\left(\boldsymbol{w}^{(i)} | \mathbf{Z}\right) .$

% \begin{equation}
% \begin{aligned}
% &\mathbb{E}_{q\left(\mathbf{Z} | \mathcal{D}\right)}\left[\log p\left(\mathcal{D}_{N | \mathbf{Z})}\right]\right.
% \\& \leq \sum_{i=1}^{N} \mathbb{E}_{q\left(\mathbf{x} | \boldsymbol{w}^{(i)}\right) q\left(\mathbf{\beta} | \boldsymbol{D}\right) q\left(\mathbf{\phi} | \boldsymbol{D}\right)}\left[\log \left(\frac{1}{N} p\left(\boldsymbol{w}^{(i)} | \mathbf{Z}\right)\right)\right] \\
% &=\sum_{i=1}^{N} \mathbb{E}_{q\left(\mathbf{x} | \boldsymbol{w}^{(i)}\right) q\left(\mathbf{\beta} | \boldsymbol{D}\right) q\left(\mathbf{\phi} | \boldsymbol{D}\right)}\left[\log p\left(\boldsymbol{w}^{(i)} | \mathbf{Z}\right)\right]-N \log N \\
% &=\sum_{i=1}^{N} \mathbb{E}_{q\left(\mathbf{x} | \boldsymbol{w}^{(i)}\right) q\left(\mathbf{\beta} | \boldsymbol{D}\right) q\left(\mathbf{\phi} | \boldsymbol{D}\right)}\left[\log p\left(\boldsymbol{w}^{(i)} | \mathbf{Z}\right)\right]
% \\
% &=\sum_{i=1}^{N} \mathbb{E}_{q\left(\mathbf{x} | \boldsymbol{w}^{(i)}\right) q\left(\mathbf{\beta} | \boldsymbol{D}\right) q\left(\mathbf{\phi} | \boldsymbol{D}\right)}\left[\log p\left(\boldsymbol{w}^{(i)} | \mathbf{x, \beta, \phi}\right)\right]
% \end{aligned}
% \end{equation}

% Where $$\mathbf{x}=\{x_1, x_2, \dots, x_N\}$$  $$q(x|w^{i}) = \prod_{k=1}^N q(x_j|w^i)$$

% $$
% \begin{aligned}
% \\
% &\mathbb{E}_{q\left(\mathbf{Z} | \mathcal{D}\right)}
% \left[\log p\left(\mathcal{D}_{N | \mathbf{Z})}\right]\right. \\&\leq \sum_{i=1}^{N} \mathbf{E}_{ q\left(\mathbf{x} | {w}^{(i)}\right) q\left(\mathbf{\phi} | {D}\right) q\left(\mathbf{\beta} | {D}\right)}\left[\log p\left(\boldsymbol{w}^{(i)} | \mathbf{x, \beta, \phi}\right)\right]
% \\
% &=\sum_{i=1 }^{N} \mathbf{E}_{\left( \prod_{j=1}^N q \left( \mathbf{x_j} | {w}^{(i)}\right)\right) q\left(\mathbf{\phi} | {D}\right) q\left(\mathbf{\beta} | {D}\right)}\left[\log p\left(\boldsymbol{w}^{(i)} | \mathbf{x, \beta, \phi}\right)\right]
% \\
% &=\sum_{i=1}^{N} \int {\left( \prod_{j=1}^N q \left( \mathbf{x_j} | {w}^{(i)}\right)\right) q\left(\mathbf{\phi} | {D}\right) q\left(\mathbf{\beta} | {D}\right)}
% \\ &\left[\log p\left(\boldsymbol{w}^{(i)} | \mathbf{x, \beta, \phi}\right)\right] d(\mathbf{x}) d(\phi) d(\beta)
% \end{aligned}
% $$

% Since $\int \prod_{j=1;j\neq i}^N\left( q\mathbf{x_j} | {w}^{(i)}\right) d(x_{j\neq i}) = 1 $ we have:
% $$
% \begin{aligned}
% \\
% &\mathbb{E}_{q\left(\mathbf{Z} | \mathcal{D}\right)}\left[\log p\left(\mathcal{D}_{N | \mathbf{Z})}\right]\right.  
% \\&\leq \sum_{i=1}^{N} \int {  q(\mathbf{x_i} | {w}^{(i)}) q\left(\mathbf{\phi} | {D}\right) q\left(\mathbf{\beta} | {D}\right)}\left[\log p\left(\boldsymbol{w}^{(i)} | \mathbf{x, \beta, \phi}\right)\right]d(\mathbf{x_i}) d(\phi) d(\beta) 
% \\
% &=\sum_{i=1}^{N} \mathbb{E}_{  q(\mathbf{x_i} | {w}^{(i)}) q\left(\mathbf{\phi} | {D}\right) q\left(\mathbf{\beta} | {D}\right)}\left[\log p\left(\boldsymbol{w}^{(i)} | \mathbf{x, \beta, \phi}\right)\right]
% \\
% &=\sum_{i=1}^{N} \mathbb{E}_{  q(\mathbf{x_i} | {w}^{(i)}) q\left(\mathbf{\phi} | {D}\right) q\left(\mathbf{\beta} | {D}\right)}\left[w_i^T \log \left(\beta p(\boldsymbol{z} | \mathbf{x_i, \phi}) \right)\right]
% \end{aligned}
% $$

% Using the reparameterization trick, we can generate: \\

% $\beta$ from $\frac{1}{N}\sum_{i=1}^N q(\beta|w^{i}) (by \; (18))$  by sampling $\epsilon_{\beta} \sim N(0, I)$; and computing $\beta=\sigma(\mu_{\beta}+\Sigma_{\beta}^{1/2}*\epsilon_{\beta})$  


% $\phi$ from$\frac{1}{N}\sum_{i=1}^N q(\phi|w^{i}) (by \; (18))$ by sampling $\epsilon_{\phi} \sim N(0, I)$; and computing $\phi=\mu_{\phi}+\Sigma_{\phi}^{1/2}*\epsilon_{\phi}$  


% $x_i$ from $q(x_i|w^i)$ by sampling $\epsilon_{x_i} \sim N(0, I)$.  and computing $x_i=\mu_{x_i}+\Sigma_{x_i}^{1/2}*\epsilon_{x_i}$  \\ 
% We can rewrite reconstruction loss as:

% \begin{equation}
% \begin{aligned}
% &\mathcal{L}\left(\phi*, \theta* | \boldsymbol{D}\right) \\&=\sum_{i=1}^{N} \mathbb{E}_{ \epsilon_\beta \sim N(0,I); \epsilon_\phi \sim N(0,I); \epsilon_{x_i} \sim N(0,I)}\left[w_i \log \left(\beta^Tp(\boldsymbol{z} | \mathbf{x_i, \phi}) \right)\right]
% \end{aligned}
% \end{equation}



% \subsection{An Upper Bound Approximation of the KL Term}



% \textbf{DKL for ${q(x|D)}$}
% $$
% \begin{aligned}
% D_{\mathrm{KL}}\left[q\left(\mathbf{x} | \mathcal{D}\right) \| p(\mathbf{x})\right]
% = D_{\mathrm{KL}}\left[q\left(\mathbf{x} | {w^1, w^2, \dots, w^N}\right) \| p(\mathbf{x})\right]
% = D_{\mathrm{KL}}\left[\frac{1}{N} \sum_{i=1}^N q\left(\mathbf{x} | {w^i}\right) \| p(\mathbf{x})\right]\\  \leq \frac{1}{N} \sum_i^N D_{\mathrm{KL}}\left[q\left(\mathbf{x} | {w^i}\right) \| p(\mathbf{x})\right]\\
% \end{aligned}
% $$
% \\
% $p(x)$ is draw from $N(x| O, (\sigma_0)^2), (\sigma_0)^2=\frac{10}{K} $ \\
% $q(x|w^i)$ is draw from $N(x| \mu_{x}^{i}, 
% (\sigma_{x}^{i})^2)$ 
% \begin{equation} \label{eq:DKLX}
% \begin{split}
% D_{\mathrm{KL}}\left[q\left(\mathbf{x} | \mathcal{D}\right) \| p(\mathbf{x})\right]
% & \leq \frac{1}{N} \sum_i^N \sum_{p=1}^2 \frac{1}{2} \left[ \frac{(\sigma_{x}^{ip})^2}{(\sigma_0)^2}+ \frac{(\mu_{x}^{ip})^2}{(\sigma_0)^2} - \log (\frac{(\sigma_{x}^{ip})^2)}{(\sigma_0)^2} - 1 \right]
% \end{split}
% \end{equation}


% %Compute DKL for q(beta)


% From the above DKL we have:


% \begin{equation}
% \begin{split}
% DKL_{prior} &\leq \mathrm{KL}_{\mathrm{approx}}^{\mathrm{UB}}
% =\sum_i^N D_{\mathrm{KL}}\left[q\left(\mathbf{x_i} | {w^i}\right) \| p(\mathbf{x_i})\right]
% \end{split}
% \end{equation}



% The network architecture for PLSV VAE is shown in Figure \ref{fig:network}. 
% W is input samples, each sample has size of V. 
% The encoder contains 4 linear layers following by softplus and Batchnorm, 
% encoder outputs $\mu$, $\sigma$ is parameters of distribution $p(X|W)$.
% Decoder part has one RBF layer to compute $\theta$ which is the topic proportion of a document and determined by the distance between its coordinate to topics coordinate ($\phi_{i=1:K}$) in visualization space.
% $\beta$ is defined by the weight of the last linear layer fc5.
